# Supplementary material for: Exploring Synergistic Ensemble Learning: Uniting CNNs, MLP-Mixers, and Vision Transformers to Enhance Image Classification
Source: arXiv:2504.09076 source file (2025-04-12)
Supplement: Supplementary file 1 [file Appendix.tex]

\newpage
